# Supplementary material for: Optical properties and charge-transfer excitations in edge-functionalized all-graphene nanojunctions
Source: arXiv:1105.2761 source file (2011-05-13)
Supplement: Supplementary file 1 [file supp-info_arxiv.pdf]

# SUPPORTING INFORMATION

# Optical properties and charge-transfer excitations in edge-functionalized all-graphene nanojunctions


Caterina Cocchi,[*,†,‡] Deborah Prezzi,[†] Alice Ruini,[†,‡] Marilia J. Caldas,[¶] and Elisa Molinari[†,‡]

*Centro S3, CNR-Istituto Nanoscienze, I-41125 Modena, Italy, Dipartimento di Fisica, Università di Modena e Reggio Emilia, I-41125 Modena, Italy, and Instituto de Física, Universidade de São Paulo, 05508-900 São Paulo, SP, Brazil*

E-mail: caterina.cocchi@unimore.it

[*]To whom correspondence should be addressed
[†]Centro S3, CNR-Istituto Nanoscienze, I-41125 Modena, Italy
[‡]Dipartimento di Fisica, Università di Modena e Reggio Emilia, I-41125 Modena, Italy
[¶]Instituto de Física, Universidade de São Paulo, 05508-900 São Paulo, SP, Brazil

# Homogeneously Functionalized Graphene Flakes

With reference to Figure 2 in the text, we report here in Table SI the molecular orbital (MO) transitions contributing to the lowest energy excitations of the homogeneously functionalized graphene nanoflakes (GNFs) considered in this work. In Figure S1 we display the isosurfaces of the MOs close to HOMO and LUMO only for the case of hydrogenated graphene flake, since the main features do not change significantly upon functionalization.

| | H- | $COCH_3$- | $NH_2$- | F- |
|---|---|---|---|---|
| E1(8) | H → L (0.90) | H → L (0.90) | H → L (0.90) | H → L (0.91) |
| E2(8) | H-3 → L (0.21)<br>H → L+1 (0.23)<br>H → L+3 (0.26) | H-3 → L (0.19)<br>H-1 → L (0.13)<br>H → L+1 (0.13)<br>H → L+2 (0.31) | H-3 → L (0.16)<br>H → L+1 (0.32)<br>H → L+3 (0.22) | H-3 → L (0.18)<br>H → L+1 (0.21)<br>H → L+2 (0.31) |
| E3(8) | H-1 → L (0.44)<br>H → L+1 (0.41) | H-1 → L (0.45)<br>H → L+1 (0.43) | H-1 → L (0.43)<br>H → L+1 (0.35) | H-1 → L (0.49)<br>H → L+1 (0.38) |

**Table SI:** Composition and weights of each transition contributing by more than 0.10 to the lowest energy excitations of functionalized graphene flakes, following the notation adopted in the text (Figure 2); H (L) indicates HOMO (LUMO).

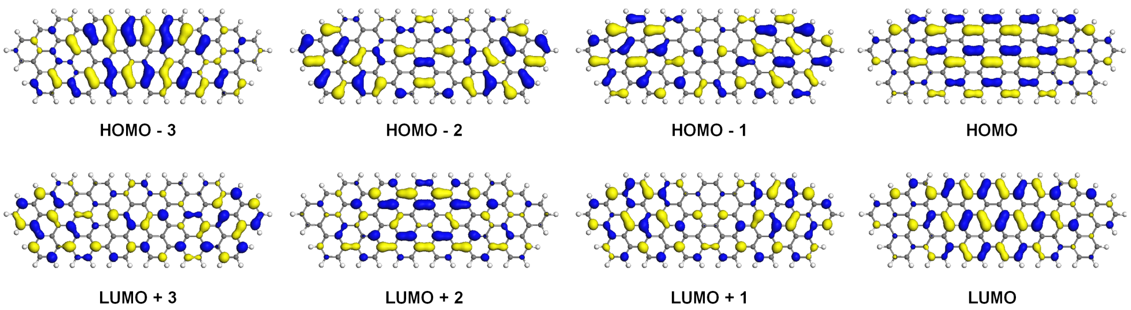


**S1:** Molecular orbitals, computed through AM1, close to HOMO and LUMO of hydrogenated graphene nanoflake.

As mentioned in the text, graphene flakes get distorted upon functionalization. In order to better estimate the effects of these distortions on the optical properties of these systems, we have taken the backbone geometry of the fully optimized $NH_2$-functionalized flake with $N = 8$ width parameter, removed the functional groups and then H-saturated the dangling bonds. The resulting structure is

shown in Figure S2(b). We have computed the optical properties of this system without any further geometrical optimization and compared them with those of a fully optimized hydrogenated flake, which is instead flat and undistorted [see Figure S2(a)]. The computed UV-Vis spectra, shown in Figure S2(c), have the same shape and the lowest energy excitations in both cases are due to the transitions reported in the first column of Table SI. An overall slight redshift is noticed in the spectrum of the distorted flake and in particular the optical gap is reduced of about 0.15 eV in this case, according to a corresponding reduction of the value of the electrical gap.

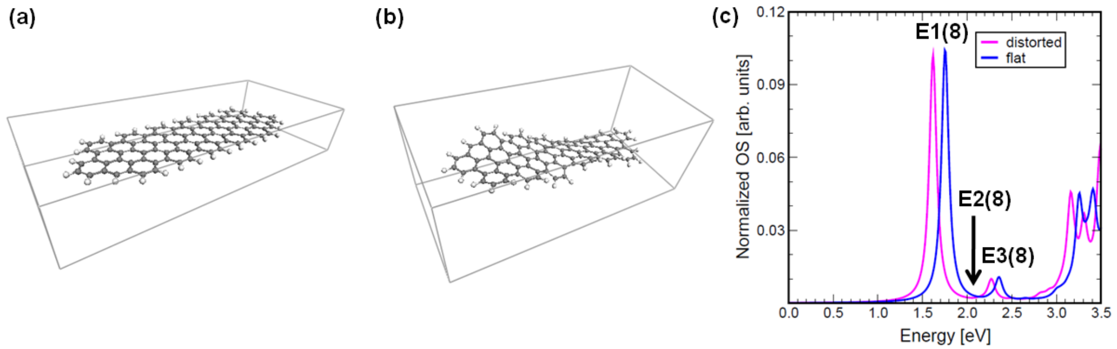


**S2:** Perspective view of hydrogenated graphene nanoflake (a) fully optimized and (b) distorted after geometrical optimization upon $NH_2$ functionalization. (c) UV-Vis spectra of the two systems: the curves represent oscillator strength (OS), normalized with respect to the number of C rings *vs.* excitation energy and are convoluted with a Lorentzian function, with a broadening of 0.05 eV.

# Graphene Nanojunctions

We report in Figure S3 the perspective view of H//$COCH_3$ and $NH_2$//F nanojunctions of width parameter $N = 8$. In Table SII the composition of the first optically active excitations is shown for all the graphene nanojunctions considered in this work. In Figure S4 localized MOs close to the frontier for the considered nanojunctions are displayed.

Analogously to Figure 4 reported in the text for the case of $NH_2$//F nanojunction, we show in Figure S5 the UV-Vis spectra and the *hole* and *electron* densities for the first optically active excitations of H//$COCH_3$ nanojunctions of width parameter $N = 6$, $N = 7$ and $N = 8$. We notice that in the case of $N = 7$ H//$COCH_3$ nanojunction, the first peak is the result of a convolution of two

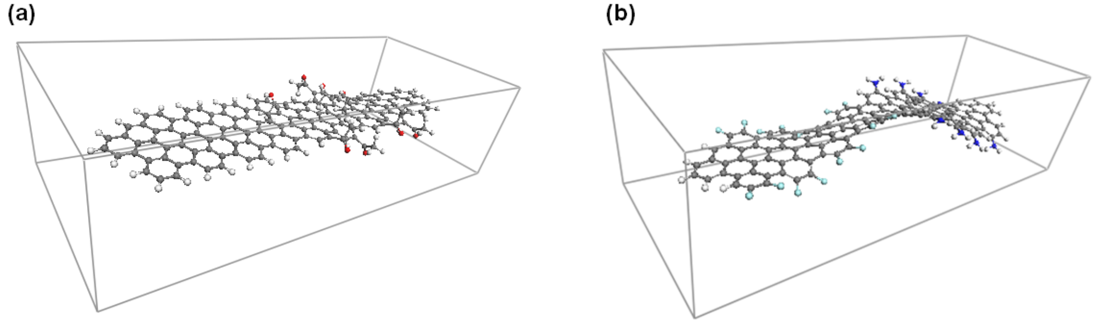


**S3:** Perspective view of the optimized structures of (a) H//$COCH_3$ and (b) $NH_2$//F nanojunctions of width parameter $N = 8$. Distortions are due to steric interactions between functional groups covalently bonded at the edges.

| | $N = 6$ | $N = 7$ | $N = 8$ |
|---|---|---|---|
| H//$COCH_3$ | H-1 → L (0.13)<br>H → L (0.24)<br>H → L+1 (0.11) | H-2 → L (0.13)<br>H-1 → L (0.11)<br>H → L (0.37) | H → L (0.81) |
| $NH_2$//H | H-2 → L (0.21)<br>H → L (0.21) | H-1 → L (0.12)<br>H → L (0.21)<br>H → L+2 (0.21)<br>H → L+3 (0.12) | H → L (0.59) |

**Table SII:** Composition and weights of each transition contributing by more than 0.10 to the lowest optically active excitation of the considered graphene nanojunctions; H (L) indicates HOMO (LUMO).

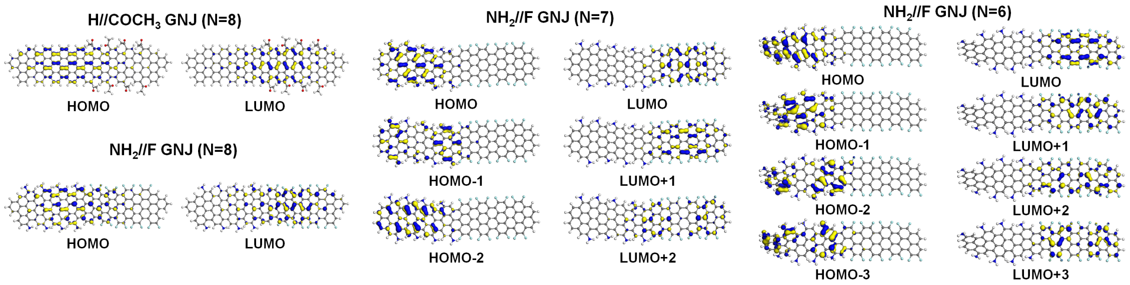


**S4:** Localized molecular orbitals, computed through AM1, of graphene nanojunctions discussed in the text. For a given structure, the symmetry of the orbitals does not change significantly by varying the functional groups. On the contrary, by varying the junction width, the electronic properties of the system are modified and accordingly the number and the shape of frontier molecular orbitals.

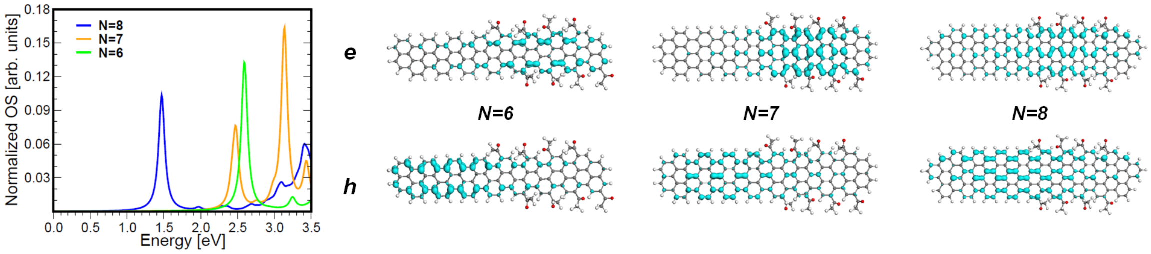


**S5:** UV-Vis spectra of width modulated H//$COCH_3$ graphene nanojunctions,, belonging to families $N = 6$, $N = 7$ and $N = 8$. The curves represent oscillator strength (OS), normalized with respect to the number of C rings *vs.* excitation energy and are convoluted with a Lorentzian function, with a broadening of 0.05 eV; Electron (*e*) and hole (*h*) probability densities are also shown for the first optically active excitations of each family.

excitations, very close in energy, only the second one presenting proper charge transfer character. We refer to this excitation in Table SII and Figure S5 as well as in Table 1 in the text. This feature is a consequence of the electronic properties of $N = 7$ *family* of hydrogenated graphene flakes, which present a dark excitation at lowest energy. In the case of H//$COCH_3$ junction the first excitation is not completely forbidden on account of the broken symmetry due to -$COCH_3$ functionalization. On the other hand, upon $NH_2$//F functionalization – which has been chosen as the most effective one – this effect disappears and the first peak is due only to the first excitation which is optically active and presents charge transfer character, as for the other considered *families*.

The trend for the UV-Vis spectra shown in Figure S5 is the same observed for $NH_2$//F nanojunctions. Also these results indicate that the flexibility of edge covalent functionalization combined with the width modulation of GNFs allow to tune the position of the first peak, still preserving its charge transfer character. The spatial localization of *hole* and *electron* densities, which quantitatively account for the charge transfer character of the excitations, are reported in Table 1 in the text for all the systems investigated in this work.
